# Supplementary material for: CBA: Contextual Quality Adaptation for Adaptive Bitrate Video Streaming (Extended Version)
Source: arXiv:1901.05712 source file (2019-01-17)
Supplement: Supplementary file 1 [file 8_appendix_notes.tex]

\clearpage
\appendices
\section{}
Generative model
\begin{align*}
    &\omega \sim p(\omega)=\GammaDis(\omega \mid 1/2, 1/2)\\
    &\phi \mid \omega \sim p(\phi \mid \omega)= \GammaDis(\phi \mid 1/2, \omega)\\
    &\pmb{\lambda}\mid \phi \sim p(\pmb{\lambda}\mid \phi)= \prod_{j=1}^D p(\lambda_j\mid \phi)=\prod_{j=1}^D \GammaDis(\lambda_j \mid b, \phi)\\
    &\pmb{\tau}\mid \pmb{\lambda} \sim p(\pmb{\tau}\mid \pmb{\lambda})= \prod_{j=1}^D p(\tau_j\mid \lambda_j)=\prod_{j=1}^D \GammaDis(\tau \mid a, \lambda_j)\\
    &\sigma^{-2} \sim p(\sigma^{-2})=\GammaDis(\sigma^{-2}\mid c_0/2,d_0/2)\\
    &\pmb{\beta} \mid \sigma^{-2}, \pmb{\tau} \sim p(\pmb{\beta}\mid \sigma^{-2},\pmb{\tau})=\prod_{j=1}^D p(\beta_j \mid \sigma^{-2},\tau_j)=\prod_{j=1}^D \NormalDis(\beta_j \mid 0, \tau_j/\sigma^{-2})\\
    &\mathbf{y}\mid \pmb{\beta}, \sigma^{-2} \sim p(\mathbf{y}\mid \pmb{\beta}, \sigma^{-2})=\NormalDis( \mathbf{y}\mid \mathbf{X}\pmb{\beta}, 1/\sigma^{-2} \mathbf{I}_t) =\prod_{i=1}^t \NormalDis( y_i \mid \mathbf{x}_i^\top \pmb{\beta}, 1/\sigma^{-2})
\end{align*}

Full Conditionals
\begin{align*}
   p(\pmb{\beta} \mid \mathbf{y}, \mathbf{X}, \sigma^{-2}, \pmb{\tau})=\NormalDis(\pmb{\beta} \mid \pmb{\mu}_{\pmb{\beta}}^{\prime}, \pmb{\Sigma}_{\pmb{\beta}}^{\prime})\\
   \pmb{\mu}_{\pmb{\beta}}^{\prime}=(\mathbf{X}^\top \mathbf{X}+ {\mathbf{T}^{\prime}}^{-1})^{-1} \mathbf{X}^\top \mathbf{y}\\
   \pmb{\Sigma}_{\pmb{\beta}}^{\prime}=1/\sigma^{-2} (\mathbf{X}^\top \mathbf{X}+ {\mathbf{T}^{\prime}}^{-1})^{-1}\\
   {\mathbf{T}^{\prime}}^{-1}=\diag(\tau_1^{-1},\dots,\tau_D^{-1})\\
   p( \sigma^{-2} \mid \mathbf{y}, \mathbf{X}, \pmb{\beta}, \pmb{\tau} )= \GammaDis(\sigma^{-2} \mid c^\prime, d^\prime)\\
   c^{\prime}=\frac{t+D+c_0}{2}\\
   d^{\prime}=\frac{(\mathbf{y}-\mathbf{X}\pmb{\beta})^\top(\mathbf{y}-\mathbf{X}\pmb{\beta})+\pmb{\beta}^\top {\mathbf{T}^{\prime}}^{-1} \pmb{\beta}+d_0}{2}\\
   p(\pmb{\tau} \mid \pmb{\beta}, \sigma^{-2}, \pmb{\lambda} ) = \prod_{j=1}^{D} \GIGDis(\tau_j \mid a-1/2, 2 \lambda_j, \beta_j^2\sigma^{-2})\\
   p(\pmb{\lambda} \mid \pmb{\tau}, \phi )=\prod_{j=1}^{D} \GammaDis(\lambda_j \mid a+b, \tau_j + \phi)\\
   p(\phi \mid \pmb{\lambda}, \omega)= \GammaDis(\phi \mid Db+1/2, \sum_{j=1}^D \lambda_j +\omega)\\
   p(\omega \mid \phi)= \GammaDis(\omega \mid 1,\phi+1)
\end{align*}
\clearpage
Generalized Inverse Gaussian 
\begin{align*}
    \GIGDis(x \mid p, a, b)= (a/b)^{p/2}(2 \mathrm{K}_{p}(\sqrt{ab}))^{-1} x^{p-1} \exp\{(ax+b/x)/2\}\\
    h(x)=1\\
    \pmb{\theta}=[p,a,b]^\top\\
    \pmb{\eta}(\pmb{\theta})=[p-1,-a/2,b/2]^\top\\
    \pmb{\theta}(\pmb{\eta})=[\eta_1+1,-2\eta_2,2\eta_3]^\top\\
    \mathbf{S}(x)=[log(x), x, 1/x]^\top\\
    A(\pmb{\eta})= \log((-\eta_2/\eta_3)^{(\eta_1+1)/2} \{2 \mathrm{K}_{\eta_1+1}(\sqrt{-4\eta_2\eta_3})\}^{-1})\\
    A(\pmb{\theta})=(a/b)^{p/2}(2 \mathrm{K}_{p}(\sqrt{ab}))^{-1}
\end{align*}
Variational Distributions
\begin{align*}
   q(\pmb{\beta})=\NormalDis(\pmb{\beta} \mid \pmb{\mu}_{\pmb{\beta}}, \pmb{\Sigma}_{\pmb{\beta}})\\
   \pmb{\mu}_{\pmb{\beta}}=(\mathbf{X}^\top \mathbf{X}+ \mathbf{T}^{-1})^{-1} \mathbf{X}^\top \mathbf{y}\\
   \pmb{\Sigma}_{\pmb{\beta}}=\langle \sigma^{-2}\rangle^{-1}  (\mathbf{X}^\top \mathbf{X}+ \mathbf{T}^{-1})^{-1}\\
   \mathbf{T}^{-1}=\diag(\langle \tau_1^{-1}\rangle,\dots,\langle \tau_D^{-1}\rangle)\\
   q( \sigma^{-2})= \GammaDis(\sigma^{-2} \mid c^\ast, d^\ast)\\
   c^{\ast}=\frac{t+D+c_0}{2}\\
   d^{\ast}=(\mathbf{y}^\top \mathbf{y} - 2\mathbf{y}^\top\mathbf{X}\langle \pmb{\beta}\rangle + \sum_{i=1}^t \mathbf{x}_i^\top \langle \pmb{\beta}\pmb{\beta}^{\top}\rangle \mathbf{x}_i  +\sum_{j=1}^D \langle \beta_j^2 \rangle \langle \tau_j^{-1} \rangle+d_0)/2\\
   q(\pmb{\tau}) = \prod_{j=1}^{D} \GIGDis(\tau_j \mid a-1/2, 2 \langle \lambda_j \rangle, \langle \beta_j^2 \rangle \langle \sigma^{-2} \rangle)\\
   q(\pmb{\lambda})=\prod_{j=1}^{D} \GammaDis(\lambda_j \mid a+b, \langle \tau_j \rangle + \langle \phi \rangle)\\
   q(\phi)= \GammaDis(\phi \mid Db+1/2, \langle \omega \rangle + \sum_{j=1}^D \langle \lambda_j \rangle)\\
   q(\omega)= \GammaDis(\omega \mid 1,\langle \phi \rangle +1)\\
   \langle \pmb{\beta}\rangle=\pmb{\mu}_{\pmb{\beta}}\\
   \langle \pmb{\beta} \pmb{\beta}^\top\rangle= \pmb{\Sigma}_{\pmb{\beta}}+\pmb{\mu}_{\pmb{\beta}}\pmb{\mu}_{\pmb{\beta}}^\top\\
   \langle \sigma^{-2} \rangle = c^\ast / d^\ast\\
   \langle \lambda_j \rangle= (a+b)/ \langle \tau_j \rangle + \langle \phi \rangle\\
   \langle \phi \rangle = (Db+1/2)/ \sum_{j=1}^D \langle \lambda_j \rangle + \langle \omega \rangle\\
   \langle \omega \rangle = 1/(\langle \phi \rangle +1)\\
   v_j=(2 \langle \lambda_j \rangle \langle \sigma^{-2} \rangle\langle \beta_j^2 \rangle)^{1/2}\\
   \langle \tau_j \rangle = \frac{(\langle \sigma^{-2} \rangle \langle \beta_j^2 \rangle)^{1/2}\mathrm{K}_{a+1/2}(v)}{(2 \langle \lambda_j \rangle)^{1/2} \mathrm{K}_{a-1/2}(v_j) } \\
   \langle \tau_j^{-1} \rangle = \frac{(2 \langle \lambda_j \rangle)^{1/2} \mathrm{K}_{3/2-a}(v)}{(\langle \sigma^{-2} \rangle \langle \beta_j^2 \rangle)^{1/2}\mathrm{K}_{1/2-a}(v) } \\
\end{align*}
\clearpage
Moments of the log conditionals
\begin{align*}
    \langle \log(p(\mathbf{y}\mid \pmb{\beta}, \sigma^{-2})) \rangle = -t/2 \log(2\pi) + t/2 \langle \log(\sigma^{-2}) \rangle - 1/2 \langle \sigma^{-2} \rangle (\mathbf{y}^\top \mathbf{y} -2\mathbf{y}^\top \langle\pmb{\beta}\rangle + \sum_{i=1}^t \mathbf{x}_i^\top \langle\pmb{\beta} \pmb{\beta}^\top \rangle \mathbf{x}_i)\\
    \langle \log(p(\pmb{\beta}\mid \sigma^{-2},\pmb{\tau})) \rangle = -D/2 \log(2\pi) + D/2 \langle \log(\sigma^{-2}) \rangle -1/2 \sum_{j=1}^D \langle\log(\tau_j)\rangle -1/2 \sum_{j=1}^D \langle \sigma^{-2} \rangle \langle \beta_j^2 \rangle \langle \tau_j^{-1}\rangle\\
    \langle \log(p(\sigma{-2}))\rangle=(c_0/2-1) \langle \log(\sigma^{-2}) \rangle -d_0/2 \langle \sigma^{-2} \rangle +c_0/2 \log(d_0/2)- log(\Gamma(c_0/2))\\
    \langle \log(p(\pmb{\tau}\mid \pmb{\lambda})) \rangle = - D \log(\Gamma(a))+ a \sum_{j=1}^D \langle\log(\lambda_j)\rangle + (a-1) \sum_{j=1}^D  \langle \log(\tau_j)\rangle - \sum_{j=1}^D \langle\lambda_j\rangle \langle\tau_j\rangle\\
    \langle \log( p(\pmb{\lambda}\mid \phi)) \rangle = - D \log(\Gamma(b)) + b D \langle \log(\phi) \rangle + (b-1)\sum_{j=1}^D \langle \log(\lambda_j) \rangle - \langle \phi \rangle \sum_{j=1}^D \langle \lambda_j \rangle\\
    \langle \log( p(\phi \mid \omega)) \rangle = \frac{1}{2} \langle \log(\omega)\rangle  - \log(\Gamma(\frac{1}{2})) - \frac{1}{2}\langle \log(\phi) \rangle  - \langle \omega \rangle \langle \phi \rangle\\
    \langle \log(p(\omega)) \rangle = \frac{1}{2} \log(\frac{1}{2}) - \log(\Gamma(\frac{1}{2})) -\frac{1}{2} \langle \log(\omega)\rangle -\frac{1}{2} \langle \omega \rangle
\end{align*}
Moments of the log variational distributions
\begin{align*}
    \langle \log(q(\pmb{\beta})) \rangle=- \frac{D}{2} \log(2\pi)- \frac{1}{2} \log(\vert \pmb{\Sigma}_{\pmb{\beta}} \vert)\\
    \langle \log(q( \sigma^{-2})) \rangle= c^\ast \log(d^\ast)-\log(\Gamma(c^\ast))+ (c^\ast-1) \langle \log(\sigma^{-2}) \rangle -d^\ast \langle \sigma^{-2} \rangle\\
    \langle \log(q(\pmb{\tau})) \rangle = (\frac{a}{2}-\frac{1}{2}) \left[p\log(2)-p\log(\langle\sigma^{-2}\rangle)+\sum_{j=1}^D\log(\langle\lambda_j\rangle) -\sum_{j=1}^D \log(\langle\beta_j^2\rangle)\right]\\
    -p\log(2)-\sum_{j=1}^D \log(\mathrm{K}_{a-\frac{1}{2}}(v))+(a-\frac{3}{2})\sum_{j=1}^D \langle\log(\tau_j)\rangle -\sum_{j=1}^D \langle \lambda_j\rangle \langle \tau_j\rangle - \frac{1}{2} \langle \sigma^{-2} \rangle \sum_{j=1}^D \langle \beta_j^2 \rangle \langle \tau_j^{-1}\rangle\\
    \langle \log(q(\pmb{\lambda})) \rangle=-D\log(\Gamma(a+b))+(a+b)\sum_{j=1}^D \log(\langle\tau_j\rangle+\langle\phi\rangle)+(a+b-1)\sum_{j=1}^D \langle\log(\lambda_j)\rangle - \sum_{j=1}^D \langle\tau_j\rangle\langle\lambda_j\rangle-\langle\phi\rangle\sum_{j=1}^D\langle\tau_j\rangle \\
    \langle \log(q(\phi)) \rangle=(D b+\frac{1}{2})\log(\langle\omega \rangle + \sum_{j=1}^D \langle \lambda_j \rangle)- \log(\Gamma(D b+\frac{1}{2})) +(D b-\frac{1}{2}) \langle \log(\phi) \rangle -\langle\omega\rangle\langle\phi\rangle- \langle\phi\rangle\sum_{j=1}^D\langle\lambda_j\rangle   \\
    \langle \log(q(\omega)) \rangle=\log(\langle \phi \rangle +1) -\langle \omega \rangle\langle \phi \rangle -\langle \omega \rangle
\end{align*}
Evidence lower bound
\begin{align*}
    \mathcal{L}=-\frac{t}{2} \log(2\pi) +\frac{c_0}{2}\log(\frac{d_0}{2})-\log(\Gamma(\frac{c_0}{2}))-c^\ast\log(d^\ast)+ log(\Gamma(c^\ast))+\sum_{j=1}^D \langle \lambda_j\rangle\langle\tau_j\rangle+\langle\phi\rangle\sum_{j=1}^D \langle\lambda_j\rangle - D\log(\Gamma(a)) \\
    - D\log(\Gamma(b)) -2 \log(\Gamma(\frac{1}{2})) +\log(2)((\frac{5}{4}-\frac{a}{2})D-\frac{1}{2})+D\log(\Gamma(a+b))+\log(\Gamma(p D+\frac{1}{2}))+\frac{1}{2}\langle\omega\rangle+\langle\omega\rangle\langle\phi\rangle+\frac{1}{2}\log(\vert \pmb{\Sigma}_{\pmb{\beta}} \vert)\\
    +(\frac{a}{2}-\frac{1}{4})(D\log(\langle\sigma^{-2}\rangle)-\sum_{j=1}^D \log(\langle\lambda_j\rangle)) +(\frac{a}{2}-\frac{1}{4})\sum_{j=1}^D \log(\langle\beta_j^2\rangle)-\sum_{j=1}^D \log(\mathrm{K}_{a-\frac{1}{2}}(v_j))-\frac{1}{2}\langle\sigma^{-2}\rangle \sum_{j=1}^D \langle\beta_j^2\rangle\langle \tau_j^{-1}\rangle\\
    -(D b+\frac{1}{2})\log(\langle\omega \rangle+\sum_{j=1}^D\langle\lambda_j\rangle)-(a+b)\sum_{j=1}^D \log(\langle\tau_j\rangle+\langle\phi\rangle)-\log(\langle\phi\rangle+1)
\end{align*}
\clearpage
transformations of the parameters 
\begin{align*}
    \pmb{\eta}_{\pmb{\beta}}=(\pmb{\Sigma}_{\pmb{\beta}}^{-1}\pmb{\mu}_{\pmb{\beta}},-\frac{1}{2}\pmb{\Sigma}_{\pmb{\beta}}^{-1}),\quad (\pmb{\mu}_{\pmb{\beta}}, \pmb{\Sigma}_{\pmb{\beta}})=(-\frac{1}{2}{\pmb{\eta}_{\pmb{\beta}}}^{-1}_2{\pmb{\eta}_{\pmb{\beta}}}_1,-\frac{1}{2} {\pmb{\eta}_{\pmb{\beta}}}^{-1}_2)\\
    {\pmb{\eta}_{\sigma^{-2}}}=(c^\ast-1, -d^\ast),\quad (c^\ast,d^\ast)=( {{{\eta}_{\sigma^{-2}}}_1}+1,- {{{\eta}_{\sigma^{-2}}}_2})\\
    {\pmb{\eta}_{\tau_j}}=(p_{\tau_j}-1, a_{\tau_j}/2, b_{\tau_j}/2),\quad (p_{\tau_j}, a_{\tau_j}, b_{\tau_j})=({{\eta}_{\tau_j}}_1+1,-2{{\eta}_{\tau_j}}_2, 2{{\eta}_{\tau_j}}_3)\\
    {\pmb{\eta}_{\lambda_j}}=(a_{\lambda_j}-1, -b_{\lambda_j}),\quad (a_{\lambda_j}, b_{\lambda_j})=({\eta_{\lambda_j}}_1+1, -{\eta_{\lambda_j}}_2)\\
    {\pmb{\eta}_{\phi}}=(a_{\phi}-1, -b_{\phi}),\quad (a_{\phi}, b_{\phi})=({\eta_{\phi}}_1+1, -{\eta_{\phi}}_2)\\
    {\pmb{\eta}_{\omega}}=(a_{\omega}-1, -b_{\omega}),\quad (a_{\omega}, b_{\omega})=({\eta_{\omega}}_1+1, -{\eta_{\omega}}_2)
\end{align*}
natural gradient
$$\hat{\nabla} f(\eta)= G(\eta)^{-1} \nabla_{\eta} f(\eta)$$
$$ \hat{\nabla}_{\eta} \mathcal{L}=\hat{\eta}-\eta$$
intermediate estimate of the natural parameters
\begin{align*}
  \hat{\pmb{\eta}}_{\pmb{\beta}}=(\langle\sigma^{-2}\rangle \mathbf{X}^\top \mathbf{y}, -\frac{1}{2} \langle \sigma^{-2}\rangle (\mathbf{X}^\top \mathbf{X}+\mathbf{T}^{-1}))\\
  \hat{\pmb{\eta}}_{\sigma^{-2}}=(\frac{t+D+c_0}{2}-1, -(\mathbf{y}^\top \mathbf{y} - 2\mathbf{y}^\top\mathbf{X}\langle \pmb{\beta}\rangle + \sum_{i=1}^t \mathbf{x}_i^\top \langle \pmb{\beta}\pmb{\beta}^{\top}\rangle \mathbf{x}_i  +\sum_{j=1}^D \langle \beta_j^2 \rangle \langle \tau_j^{-1} \rangle+d_0)/2)\\
  \hat{\pmb{\eta}}_{\tau_j}=(a-\frac{3}{2}, -\langle \lambda_j \rangle, \langle \beta_j^2 \rangle \langle\sigma^{-2}\rangle/2)\\
  \hat{\pmb{\eta}}_{\lambda_j}=(a+b-1, -\langle\tau_j\rangle-\langle\phi\rangle)\\
  \hat{\pmb{\eta}}_{\phi}=(D b -\frac{1}{2},-\langle\omega\rangle -\sum_{j=1}^D \langle\lambda_j\rangle)\\
  \hat{\pmb{\eta}}_{\omega}=(0,-\langle\phi\rangle-1)
\end{align*}
\newpage
\hspace{1cm}
\newpage
